# Supplementary material for: The Gate Always Closes: On Injecting Auxiliary Signals into Frozen Vision-Language Models
Source: arXiv:2607.23335 source file (2026-11-01)
Supplement: Supplementary file 1 [file supp.tex]

\makeatletter
\ifdefined\@writefile\else
\makeatother

\documentclass[runningheads]{llncs}

% ---------------------------------------------------------------
% \usepackage[review,year=2026,ID=458]{accv}
\usepackage[year=2026]{accv}

% ---------------------------------------------------------------
\usepackage{accvabbrv}
\usepackage{graphicx}
\usepackage{booktabs}
\usepackage{multirow}
\usepackage{amsmath,amssymb}
\usepackage{mathtools}
\usepackage{bm}
\usepackage[accsupp]{axessibility}
\usepackage{subcaption}
\usepackage{xcolor}
\usepackage[pagebackref,breaklinks,colorlinks,citecolor=accvblue]{hyperref}
\usepackage{xr-hyper}
\externaldocument{main}
\usepackage{orcidlink}

\usepackage{xcite}
\externalcitedocument{main} % মেইন ফাইলের সাইটেশন ডাটা লিংক করা হলো
% ---------------------------------------------------------------
\newcommand{\Ln}{\mathbb{L}^{n}_{\kappa}}

\newcommand{\linner}[2]{\langle #1, #2 \rangle_{\mathcal{L}}}

% ---------- page-fit engineering (spacing around floats) ----------
\setlength{\textfloatsep}{6pt plus 2pt minus 2pt}
\setlength{\intextsep}{6pt plus 2pt minus 2pt}
\setlength{\dbltextfloatsep}{6pt plus 2pt minus 2pt}
\setlength{\floatsep}{6pt plus 2pt minus 2pt}
\setlength{\abovecaptionskip}{4pt}
\setlength{\belowcaptionskip}{0pt}

% ---------- Supplementary numbering: S-prefix on floats and sections ----------
\setcounter{figure}{0}
\setcounter{table}{0}
\setcounter{section}{0}

\renewcommand{\thetable}{S\arabic{table}}

\begin{document}
\makeatletter
\fi
\makeatother
\title{Supplementary Material: \texorpdfstring{``The Gate Always Closes: On Injecting Auxiliary Signals into Frozen Vision-Language Models''}{The Gate Always Closes}}
\titlerunning{Supplementary Material}

% \author{Anonymous}
% \authorrunning{Anonymous}
% \institute{Anonymous Institution}
\author{
Moshiur Farazi\inst{1}
\and
Sameera Ramasinghe\inst{2}
\and
Bekir Sait Ciftler\inst{1}
\and
Mahbub Ahmed Turza\inst{3}
\and
Shafin Rahman\inst{3}
}

\institute{
University of Doha for Science and Technology, Doha, Qatar
\and
Pluralis Research, Australia
\and
North South University, Dhaka, Bangladesh
}

\maketitle

% =====================================================
% Guide to the Supplementary
% =====================================================
\noindent This document supplements the main paper. Section, figure, and table numbers are prefixed with \textbf{S}; citations use the same bibliography as the main paper. The sections below are ordered to mirror the main paper's flow, so a reader who wants to expand any specific claim can find its supplement in the same reading order.

\medskip

\noindent\textbf{Guide to the Supplementary.}
\begin{center}
\scalebox{0.92}{
\begin{tabular}{@{}p{0.42\linewidth}p{0.50\linewidth}@{}}
\toprule
\textbf{Supplementary section} & \textbf{Extends this part of the main paper} \\
\midrule
\ref{supp:sec:related}: Extended Related Work & Section~1 (Introduction), positioning paragraph \\
\ref{supp:sec:geom}: Extended Geometric Primitives & Section~2 (Experimental Vehicle), Sec.~2.1--2.2 \\
\ref{supp:sec:training}: Training and Compute Details & Section~2.4 (Training setup) \\
\ref{supp:sec:ablations}: Behavioural Ablations of the Auxiliary Pathway & Section~3 (Suppression Phenomenon), Table~1 of main \\
\ref{supp:sec:gate}: Gate Trajectories During Training & Section~3.2 and Fig.~2 of main \\
\ref{supp:sec:sc_breakdown}: Per-Category SugarCrepe Breakdown & Section~5 (Experimental Results), the SC average line \\
\ref{supp:sec:generation}: Generation-Side Evaluation (POPE, COCO) & Section~5.3 (Generation Safety) \\
\ref{supp:sec:discussion}: Extended Discussion & Section~6 (Conclusion), tail pointer \\
\ref{supp:sec:limitations}: Limitations & Section~6 (Conclusion), the Limitations sentence \\
\bottomrule
\end{tabular}}
\end{center}

\medskip

% =====================================================
\section{Extended Related Work}
\label{supp:sec:related}
% =====================================================

The Introduction of the main paper lists the six threads closest to this work in one paragraph and points here for the fuller treatment. This section expands each thread and positions our contribution against it.

\noindent\textbf{Prefix and prompt tuning.}
VPT~\cite{jia2022vpt} introduced learned prefix tokens for vision transformers, and LLaMA-Adapter~\cite{gao2023llamaadapter} carried the idea into LLM layers with zero-initialised gating. In both cases the prefix content is learned end-to-end via backpropagation through the frozen backbone. Different to these works, we ask what happens when the prefix content is derived from a structured external computation --- here a geometric relational graph --- rather than shaped by the task gradient itself. We find that the structured pathway is reliably suppressed under a task-only loss.

\noindent\textbf{Auxiliary signal injection in VLMs.}
A growing body of work attaches scene-graph generators and feeds predicate triplets as text~\cite{wang2024llavassg,mitra2024ccot,herzig2023structured}, injects visual relation encodings as prefix tokens~\cite{hypervis2026}, or modulates attention weights with structural biases. Yang \etal~\cite{yang2026scenegraph_thinking} instead use scene graphs as reinforcement signals. These efforts differ in what they inject, but a common design assumption is that a well-shaped auxiliary signal will be consumed at inference. Our investigation spans two injection mechanisms (attention bias and prefix tokens) and characterises the conditions under which the pathways carrying that signal remain active or become suppressed.

\noindent\textbf{Hyperbolic VLMs.}
Hyperbolic spaces embed hierarchical structure with low distortion~\cite{nickel2017poincare,ganea2018hyperbolicnn,he2025hyperbolic_survey}. MERU~\cite{desai2023meru} introduced hyperbolic contrastive VLMs, and HyCoCLIP~\cite{pal2025hycoclip} extended this with compositional entailment. Ramasinghe \etal~\cite{ramasinghe2024accept} showed that geodesic contrastive losses conflict with entailment cones and cause curvature collapse; our angle-based losses inherit this insight. HyperET~\cite{peng2025hyperet} demonstrated efficient hyperbolic training for MLLMs. In our experiments the Lorentz manifold serves as the experimental vehicle for generating the auxiliary signal. The suppression and norm-mismatch findings, however, are mechanism-level rather than geometry-level, and would apply equally to any structured signal delivered through an analogous pathway.

\noindent\textbf{Structured attention biases.}
ALiBi~\cite{press2022alibi} and RoPE~\cite{su2024rope} inject position-dependent biases into attention, and FlashBias~\cite{wu2025flashbias} provides efficient kernels for dense variants. Dalal \etal~\cite{dalal2026attwarp} improve LLaVA's compositionality through attention-guided image warping. Our attention-bias mechanism is a special case of this family, and the suppression finding applies to it directly.

\noindent\textbf{Compositionality benchmarks.}
ARO~\cite{yuksekgonul2023aro}, Winoground~\cite{thrush2022winoground} and SugarCrepe~\cite{hsieh2024sugarcrepe} probe compositional understanding. SugarCrepe++ addresses known text-only biases in the original benchmark~\cite{dumpala2024sugarcrepepp}. SCRAMBLe~\cite{mishra2025scramble} reaches 54.8\% Winoground group via preference tuning. Our evaluation uses SugarCrepe (7 subcategories) and Winoground; we note the known biases where they bear on the interpretation.

\noindent\textbf{Auxiliary noise as regularisation.}
NEFTune~\cite{jain2024neftune} showed that adding uniform noise to input embeddings during instruction tuning improves downstream evaluation scores. This raises the possibility that part of the benefit attributed to structured auxiliary signals is captured by generic noise perturbation. We control for this confound with the fixed-random prefix baseline (G2) in the main paper's results section.

% =====================================================
\section{Extended Geometric Primitives}
\label{supp:sec:geom}
% =====================================================

The main paper Sec.~2.1 uses several hyperbolic-geometry primitives (manifold, exponential map, entailment cone, central angle, Einstein midpoint) by name only. This section gives their explicit forms.

\noindent\textbf{Lorentz manifold.} The Lorentz model $\Ln$ is the upper sheet of the hyperboloid in $(n{+}1)$-dimensional Minkowski spacetime ($n{=}256$):
\begin{equation}
\Ln = \left\{\mathbf{p} \in \mathbb{R}^{n+1} : \linner{\mathbf{p}}{\mathbf{p}} = -\frac{1}{\kappa},\; p_0 > 0\right\},
\label{supp:eq:lorentz}
\end{equation}
where the Lorentzian inner product is $\linner{\mathbf{p}}{\mathbf{q}} = -p_0 q_0 + \sum_{i=1}^n p_i q_i$ and $\kappa > 0$ is the learnable curvature parameter (initialised at 1.0, clamped to $[0.1, 5.0]$). Tangent vectors at the origin have their time component fixed at $v_0=0$.

\noindent\textbf{Exponential map at the origin.} The exponential map at $\mathbf{o} = (\sqrt{1/\kappa}, 0, \ldots, 0)^\top$ sends a tangent vector $\mathbf{v}$ (with $v_0{=}0$) to a manifold point:
\begin{equation}
\exp_\mathbf{o}^\kappa(\mathbf{v}) = \cosh\!\left(\sqrt{\kappa}\|\tilde{\mathbf{v}}\|\right)\mathbf{o} + \frac{\sinh(\sqrt{\kappa}\|\tilde{\mathbf{v}}\|)}{\sqrt{\kappa}\|\tilde{\mathbf{v}}\|}\mathbf{v},
\label{supp:eq:expmap}
\end{equation}
followed by manifold projection $p_0 \leftarrow \sqrt{1/\kappa + \|\tilde{\mathbf{p}}\|^2}$, where $\tilde{\mathbf{p}} = (p_1, \ldots, p_n)$ denotes the spatial coordinates.

\noindent\textbf{Central angle.} Two points $\mathbf{p}, \mathbf{q}$ are separated by the central angle at the origin
\begin{equation}
\phi(\mathbf{p}, \mathbf{q}) = \arccos\!\left(\frac{\langle \tilde{\mathbf{u}}_\mathbf{p},\, \tilde{\mathbf{u}}_\mathbf{q} \rangle}{\|\tilde{\mathbf{u}}_\mathbf{p}\|\;\|\tilde{\mathbf{u}}_\mathbf{q}\|}\right),
\label{supp:eq:angle}
\end{equation}
where $\tilde{\mathbf{u}}_\mathbf{p}$ is the spatial part of $\log_\mathbf{o}^\kappa(\mathbf{p})$.

\noindent\textbf{Entailment cone half-aperture.} Every point $\mathbf{q}\in\Ln$ with $\|\tilde{\mathbf{q}}\|\ge K$ defines an entailment cone with half-aperture
\begin{equation}
\omega(\mathbf{q}) = \arcsin\!\left(\frac{K}{\|\tilde{\mathbf{q}}\|}\right), \qquad K{=}0.1.
\label{supp:eq:aperture}
\end{equation}
The cone containment test $\phi(\mathbf{p},\mathbf{q}) \le \omega(\mathbf{q})$ is inherently asymmetric because different points carry different apertures --- points closer to the origin have larger $\omega(\mathbf{q})$ and therefore contain more of the manifold, matching the intended semantics that general concepts contain specific ones.

\noindent\textbf{Einstein midpoint (aggregation).} Per-node embeddings are computed from per-edge relation tangents via the Einstein midpoint~\cite{ungar2005analytic}. Denoting the manifold-mapped edge embeddings for node $i$ as $\{\mathbf{z}_{ij}\}_{j=1}^N$ with time components $\gamma_{ij} = z_{ij,0}$, the weighted Minkowski sum is
\begin{equation}
\mathbf{z}_i^{\text{raw}} = \frac{\sum_{j=1}^N \gamma_{ij}\,\mathbf{z}_{ij}}{\left|\sum_{j=1}^N \gamma_{ij}\right|},
\qquad \mathbf{z}_i = \text{proj}_{\Ln}\!\big(\mathbf{z}_i^{\text{raw}}\big),
\label{supp:eq:einstein}
\end{equation}
where the projection restores $z_{i,0} = \sqrt{1/\kappa + \|\tilde{\mathbf{z}}_i^{\text{raw}}\|^2}$. Weighting by the time component (rather than uniformly) is what distinguishes the Einstein midpoint from a naive Minkowski average and is what preserves the hyperbolic geometry under aggregation.

\noindent\textbf{Relative geometry encoding.} The relative geometry between region proposals $i$ and $j$ is encoded from centre offsets and log size ratios:
\begin{equation}
\Delta_{ij} = \left[\tfrac{x_i - x_j}{w_j},\, \tfrac{y_i - y_j}{h_j},\, \log\tfrac{w_i}{w_j},\, \log\tfrac{h_i}{h_j}\right] \in \mathbb{R}^4.
\label{supp:eq:spatial}
\end{equation}
This four-dimensional per-pair feature is concatenated with the RoI-feature pair and fed into the spatially-biased multi-head self-attention that produces the dense relation tensor $\mathbf{R}\in\mathbb{R}^{N\times N\times d}$.

\noindent\textbf{RMS text-mean rescaling.} The prefix-token rescaling of the main paper's Eq.~(4) is, in fully explicit form, applied to any projected prefix token $\mathbf{t} \in \mathbb{R}^{d_{\text{llm}}}$ as
\begin{equation}
\hat{\mathbf{t}} = \mathrm{RMSNorm}(\mathbf{t}) \cdot \frac{\|\bar{\mathbf{e}}\|_2}{\|\mathrm{RMSNorm}(\mathbf{t})\|_2},
\label{supp:eq:rmsfix}
\end{equation}
where $\bar{\mathbf{e}}$ is the mean text embedding vector in the batch. The result is a prefix whose L2-norm distribution tracks that of the text embeddings.

\noindent\textbf{Numerical stability notes.} All the primitives above have edge cases that produce NaNs under naive floating-point implementation. We clamp the tangent-vector norm to $[10^{-6}, 5]$ before every $\exp$ map to avoid both underflow in $\sinh(\cdot)/\|\tilde{\mathbf{v}}\|$ and overflow in $\cosh$. The $\arccos$ argument in Eq.~\ref{supp:eq:angle} is clamped to $[-1+10^{-6}, 1-10^{-6}]$ to protect its derivative. The curvature $\kappa$ is clamped to $[0.1, 5.0]$ per gradient step; a hinge penalty $\mathcal{L}_\kappa=\max(0, 0.3-|\kappa|)^2$ discourages $\kappa$ from approaching the lower bound, which would blow up the cone half-apertures.

% =====================================================
\section{Training and Compute Details}
\label{supp:sec:training}
% =====================================================

The main paper Sec.~2.4 sketches the training setup in one paragraph. This section gives the full recipe --- hyperparameters, optimizer groups, compute cost --- so an implementer can reproduce the reported numbers.

\begin{table}[t]
\centering
\caption{Full training recipe for the headline configurations. Values are shared across configurations unless noted. Per-configuration deltas (e.g., $\alpha_{\max}$ for the two attention-bias runs, prefix dropout for the two prefix runs) are indicated inline in the main paper Sec.~3.1 demonstrations.}
\label{supp:tab:hyperparams}
\scalebox{0.86}{
\begin{tabular}{ll}
\toprule
\textbf{Group} & \textbf{Setting} \\
\midrule
Backbone & LLaVA-1.5-7B (frozen weights) \\
LoRA rank & 16 (query and value projections only) \\
Optimizer (LoRA) & AdamW, learning rate $2\times 10^{-5}$, weight decay 0 \\
Optimizer (graph) & Riemannian Adam~\cite{geoopt}, learning rate $10^{-4}$ \\
Optimizer ($\kappa$) & Vanilla Adam, learning rate $10^{-4}$, no gradient clipping \\
\midrule
Batch size (per GPU) & 8 \\
Gradient accumulation & 2 (effective batch $16 \times$ 8 GPUs $= 128$) \\
Precision & bfloat16 \\
Training data & GQA \texttt{train\_balanced}, $\approx$82K samples \\
Epochs & 5 (3 for ablations, marked in captions) \\
Warmup & 100 steps linear ramp on $\alpha(t)$ from $0.001$ to $\alpha_{\max}$ \\
\midrule
Manifold dimension & $n = 256$ \\
Number of region proposals & $N = 36$ \\
RoI feature dimension & $d_v = 1024$ (CLIP ViT-L, before projector) \\
Prefix tokens (Mechanism B) & $K = 4$ \\
Prefix dropout & $p = 0.5$ (except S4 which sets $p = 0$) \\
Cone half-aperture constant & $K_\omega = 0.1$ (in Eq.~\ref{supp:eq:aperture}) \\
Curvature bounds & $\kappa \in [0.1, 5.0]$, initialised at $1.0$ \\
\bottomrule
\end{tabular}}
\end{table}

\noindent\textbf{Optimizer group separation.} The three optimizer groups matter for stability. Putting the LoRA weights and the hyperbolic-graph parameters under the same optimizer causes the graph to run at the LoRA learning rate ($2\times 10^{-5}$), which is 5$\times$ too small for the geometric losses to converge within the training budget. Putting the curvature $\kappa$ under Riemannian Adam causes it to over-shoot the $[0.1, 5.0]$ interval because the Riemannian correction inflates its step size near the lower bound. Using a vanilla Adam for $\kappa$ alone, without gradient clipping, was the setting under which $\kappa$ reliably stabilised near its initialised value.

\noindent\textbf{Compute cost.} Every headline configuration was trained on 8$\times$A100 80GB. End-to-end wall-clock times (training + full-testdev eval) were approximately: RMS-prefix ungated 14h, attention-bias configurations 9h each ($\alpha_{\max}$ affects gradient budget but not wall-clock), soft-prompt 8h (fewest active parameters), Euclidean 9h, G2 ablation 18h (longest because it inherits the RMS-prefix architecture without benefit of the geometric-loss regularisation, so more epochs were needed to converge), synthesis 12h. Full-testdev GQA evaluation is 45--60 min per configuration on a single A100. VSR and Winoground evaluations are $<$5 min each. COCO captioning on val2017 is $\approx$30 min per configuration with greedy decoding.

\noindent\textbf{Reproducibility.} Every configuration is a single training run under one fixed seed. This is a known limitation --- see Sec.~\ref{supp:sec:limitations}. Full checkpoints and evaluation scripts will be released at anonymised URL upon acceptance.

% =====================================================
\section{Behavioural Ablations of the Auxiliary Pathway}
\label{supp:sec:ablations}
% =====================================================

The main paper Sec.~3 (Suppression Phenomenon) argues that every learnable gated pathway in the five configurations S1--S5 is \emph{behaviourally closed} --- the model's output distribution treats the auxiliary pathway as noise. Table~\ref{supp:tab:ablations} below reports the per-configuration numbers behind this claim: task accuracy with the pathway active versus removed at inference.

\begin{table}[t]
\centering
\caption{Behavioural ablations of the auxiliary pathway at inference. Task accuracy with the pathway active vs.\ removed (attention bias zeroed for S1--S2; prefix tokens dropped for S4--S5). Every $|\Delta|$ sits within 1.3pp of no-op, and S5's negative $\Delta$ shows the pathway is worse than no injection --- the operational meaning of \emph{behaviourally closed}. S3 has no active pathway at inference (softplus$(-8.5){\approx}0$), so ablation is a no-op.}
\label{supp:tab:ablations}
\scalebox{0.85}{
\begin{tabular}{lcccl}
\toprule
\textbf{Config} & \textbf{Gate/scale} & \textbf{With pathway} & \textbf{Without pathway} & \textbf{$\Delta$} \\
\midrule
S1 (Attn bias, $\alpha{=}0.05$) & $\beta{=}{-}0.70$ & 58.05 & 57.98 & $+$0.07 \\
S2 (Attn bias, $\alpha{=}0.01$)\textsuperscript{$\dagger$} & $\beta{=}{-}0.58$ & 60.40 & 60.65 & $-$0.25 \\
S3 (Margin, LoRA frozen) & $\beta{=}{-}8.5$ (${\approx}0$) & \multicolumn{2}{c}{pathway inactive by design} & --- \\
S4 (Prefix, no dropout)\textsuperscript{$\dagger$} & $\gamma{=}{-}0.35$ & 59.40 & 60.05 & $-$0.65 \\
S5 (Raw prefix gated)\textsuperscript{$\dagger$} & $\gamma{=}{+}0.005$ & 59.35 & 60.60 & $-$1.25 \\
\bottomrule
\end{tabular}}
\par\smallskip
\footnotesize\textsuperscript{$\dagger$}Reported on a 2{,}000-question testdev subset; other cells on full testdev.
\end{table}

All ablation deltas fall within 1.3pp, and four of the five within $\pm 0.5$pp. Ablating the pathway at inference does not restore compositional signal to the LLM; in the S5 case it \emph{improves} accuracy, indicating that the learned prefix is worse than no injection at all. This is the operational content of ``behaviourally closed'': the model's output distribution has learned to treat the auxiliary pathway as noise, whether the gate parameter itself sits near zero (S3, S5) or at a value that would nominally pass a substantial fraction of the signal (S1, S2, S4).

\noindent\textbf{What ``ablation'' means per mechanism.} For attention-bias configurations (S1, S2), ablating means setting $\mathbf{B}$ to the zero matrix at inference; the LLM sees no additive bias on the image-patch causal mask, only the standard causal structure. For prefix configurations (S4, S5), ablating means dropping the $K{=}4$ prefix tokens from the input sequence entirely; the LLM sees only the image patches followed by the caption tokens. S3's ablation is a no-op because $\mathrm{softplus}(-8.5){\approx}2\times 10^{-4}$ already reduces the pathway to numerical noise. In all cases the LoRA weights are untouched --- the ablation isolates the inference-time contribution of the auxiliary pathway from the training-time regularisation effect the pathway induced on LoRA.

\noindent\textbf{Why the numbers are close but not identical.} A perfectly behaviourally-closed pathway would produce $\Delta = 0$ exactly. The observed $|\Delta|$ values of 0.07--1.25pp reflect two effects. First, floating-point non-associativity when the bias tensor is added and then removed does not exactly cancel across all 32 layers. Second, in the S5 case, the residual contribution of the raw prefix embeddings is large enough that the LLM's LoRA weights have compensated by shifting slightly, so removing the prefix at inference leaves a residual drift that hurts more than it helps.

% =====================================================
\section{Gate Trajectories During Training}
\label{supp:sec:gate}
% =====================================================

The main paper (Sec.~3.2 and Fig.~2) shows the gate parameters at convergence. Here we plot the full trajectories, contrasting the five suppressed configurations with the Euclidean variant whose gate stays open at a measurable GQA cost.

\begin{figure}[t]
    \centering
    \begin{minipage}[c]{0.5\linewidth}
        \includegraphics[width=\linewidth]{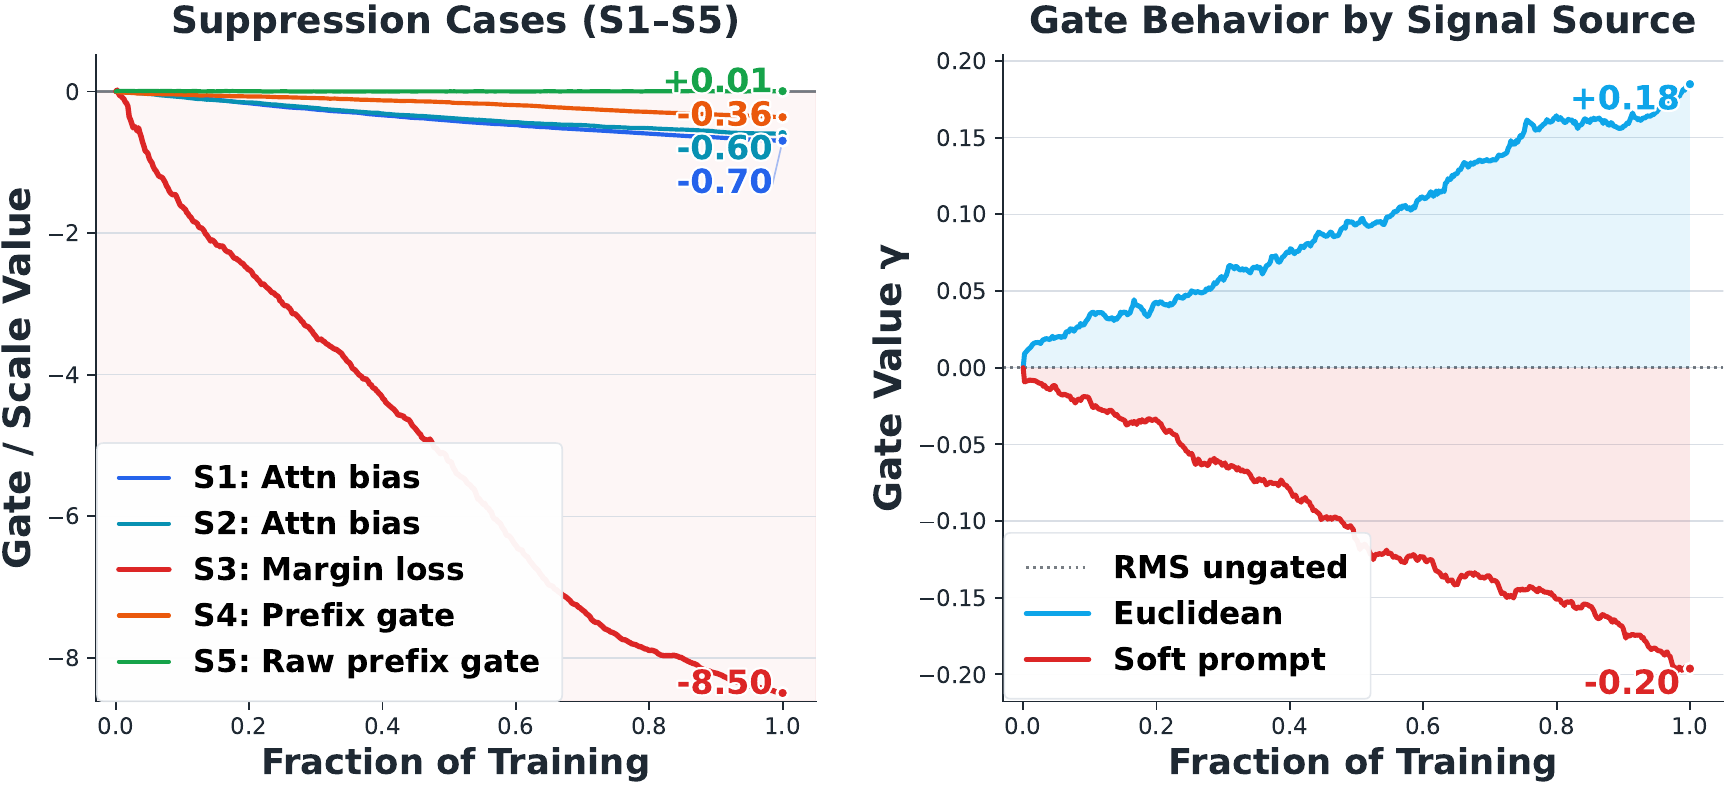}
    \end{minipage}%
    \hfill
    \begin{minipage}[c]{0.46\linewidth}
        \caption{Gate dynamics over training. \textbf{Left:} the five suppressed gates, all behaviourally closed (Table~\ref{supp:tab:ablations}); three drift to modest negatives, one dives to $-8.5$, one hovers near zero. \textbf{Right:} the Euclidean variant is the only one whose gate stays positive ($\gamma{=}+0.19$), yet its GQA drops to 59.15\% (vs.\ 60.38\% baseline); the soft-prompt gate goes negative ($\gamma{=}-0.20$) with no geometric backbone to keep it open.}
        \label{supp:fig:gate_comparison}
    \end{minipage}
\end{figure}

The trajectories corroborate the two-regime story in the main paper: gates in the dead-gradient regime drift slowly toward small negatives (S1, S2, S4), while a gate in the negative-utility regime is driven hard toward large negatives (S3, at $-8.5$). The Euclidean variant is the exception that clarifies the rule --- its gate does stay positive, but the pathway it admits actively costs 1.23pp on GQA, so ``open'' is not the same as ``useful''.

% =====================================================
\section{Per-Category SugarCrepe Breakdown}
\label{supp:sec:sc_breakdown}
% =====================================================

The main paper's results section summarises SugarCrepe as a single average. Here we decompose that average across the seven categories (Replace-Object/\allowbreak Attribute/\allowbreak Relation, Swap-Object/\allowbreak Attribute, Add-Object/\allowbreak Attribute) to expose which perturbations each variant handles.

\begin{figure*}[!t]
\centering

\begin{minipage}[t]{0.48\linewidth}
    \centering
    \includegraphics[width=\linewidth]{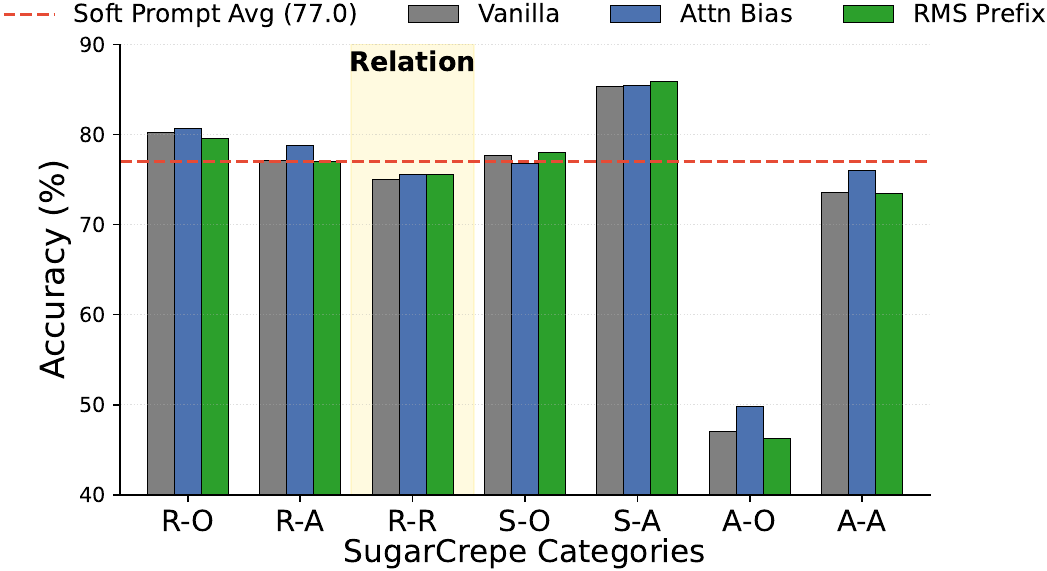}
    \vspace{-1.5em}
    \caption{SugarCrepe accuracy per category, all seven perturbation types. The attention-bias variant (small $\alpha$) peaks on Add-Object ($+2.82$pp) and Add-Attribute ($+2.46$pp) relative to vanilla LLaVA-1.5, consistent with the hierarchical containment signal the entailment cones are trained on. The soft-prompt control, despite carrying no geometric backbone, attains the highest average --- reinforcing the caution from the main paper that the average alone is a poor summary.}
    \label{supp:fig:sc_breakdown}
\end{minipage}
\hfill
\begin{minipage}[t]{0.50\linewidth}
    \centering
    \vspace{-4em}

    \refstepcounter{table}
    \label{supp:tab:sc_detail}

    \begin{minipage}{\linewidth}
        \footnotesize
        \textbf{Table~\thetable:} SugarCrepe per-category accuracy. R: Replace, S: Swap, A: Add. G2 = Hyp.\ prefix with the geometric losses removed (cf.\ main paper Table~3). Numbers are strict SugarCrepe accuracy under log-likelihood scoring; bolded row marks the per-column best.
    \end{minipage}

    \vspace{6pt}

    \resizebox{\linewidth}{!}{%
    \begin{tabular}{lccccccc|c}
    \toprule
    \textbf{Method} & \textbf{R-O} & \textbf{R-A} & \textbf{R-R} & \textbf{S-O} & \textbf{S-A} & \textbf{A-O} & \textbf{A-A} & \textbf{Avg} \\
    \midrule
    Vanilla & 80.21 & 77.16 & 74.96 & 77.64 & 85.29 & 46.99 & 73.55 & 73.69 \\
    Attn.\ bias (small $\alpha$) & 81.11 & 79.31 & 77.31 & 78.86 & 86.04 & 50.73 & 76.73 & 75.73 \\
    RMS prefix, ungated & 79.54 & 77.03 & 75.60 & 78.05 & 85.89 & 52.62 & 74.71 & 74.78 \\
    Soft prompt & 81.60 & 80.71 & 77.81 & 80.08 & 86.04 & 53.73 & 79.05 & 77.00 \\
    \textbf{Hyp.\ prefix, no geo.\ (G2)} & \textbf{83.17} & \textbf{81.73} & \textbf{78.88} & \textbf{80.89} & \textbf{86.94} & \textbf{58.20} & \textbf{82.08} & \textbf{78.84} \\
    \bottomrule
    \end{tabular}}
\end{minipage}

\end{figure*}

The category-level breakdown makes two things visible that the average hides. First, the attention-bias variant is not uniformly stronger than vanilla; its gain is concentrated on the Add perturbations, exactly where a containment-hierarchy signal would be expected to help. Second, the G2 row (hyperbolic prefix trained without the geometric losses) tops every column despite the ablation removing the geometry --- consistent with the main paper's argument that the prefix pathway is not what carries the compositional signal at inference.

% =====================================================
\section{Generation-Side Evaluation: POPE and COCO Captioning}
\label{supp:sec:generation}
% =====================================================

The main paper Sec.~5.3 (Generation Safety) reports the headline finding --- that RMS-normed prefix injection preserves POPE within noise but loses 0.036 CIDEr, and that the soft-prompt variant drops much further (CIDEr 0.987 vs.\ 1.132) despite its POPE score matching vanilla. The full per-condition table is below.

\begin{table}[t]
\centering
\caption{Generation-side evaluation across the four LLaVA-1.5 configurations. POPE reports accuracy (\%) on the random, popular, and adversarial object-existence probes (the three splits stress increasingly biased distractor sampling). Captioning is COCO val2017 (5{,}000 images), greedy decoding, pycocoevalcap; SPICE is omitted because of a Java version incompatibility in the local eval harness. Best per column in bold. The soft-prompt row is the case where a POPE-clean method is still generation-degraded on captioning --- a reminder that POPE alone underestimates generation harm.}
\label{supp:tab:generation}
\scalebox{0.78}{
\begin{tabular}{lcccccc}
\toprule
& \multicolumn{3}{c}{\textbf{POPE (\%)}} & \multicolumn{3}{c}{\textbf{COCO captioning}} \\
\cmidrule(lr){2-4} \cmidrule(lr){5-7}
\textbf{Method} & rand.\ & popular & adv.\ & BLEU-4 & METEOR & CIDEr \\
\midrule
LLaVA-1.5 vanilla & 86.30 & 85.13 & 83.40 & \textbf{0.324} & \textbf{0.280} & \textbf{1.132} \\
\quad + RMS prefix, ungated (hyp.) & 83.97 & 83.30 & 82.30 & 0.321 & 0.259 & 1.096 \\
\quad + Attn.\ bias (small $\alpha$) & 86.30 & 85.53 & 84.13 & 0.314 & 0.255 & 1.069 \\
\quad + Soft prompt (no geometry) & \textbf{86.63} & \textbf{85.90} & \textbf{84.20} & 0.287 & 0.235 & 0.987 \\
\bottomrule
\end{tabular}}
\end{table}

Two secondary observations follow from the full table. First, the attention-bias variant is generation-safe on POPE (adversarial split slightly above vanilla at 84.13\% vs.\ 83.40\%) but still loses 0.063 CIDEr, so even a design that never enters the residual stream directly is not free on fluency. Second, the RMS-prefix row is the only configuration with a POPE drop on the random split (83.97\% vs.\ 86.30\%), yet its captioning metrics are closer to vanilla than the soft prompt's --- an ordering that any single generation benchmark, taken alone, would obscure.

\noindent\textbf{POPE subset construction.} POPE probes ``Is there an X in the image?'' where X is either a positive (present) or a distractor (absent) object. The three splits differ in how distractors are sampled: \emph{random} draws distractors uniformly from the COCO label set, \emph{popular} biases toward objects that frequently co-occur with the present objects in COCO, and \emph{adversarial} explicitly picks distractors that are semantically near the present objects. Adversarial is the hardest split, so a drop concentrated there indicates the model is less discriminating between semantically similar objects.

\noindent\textbf{Why the RMS-prefix POPE drop is not a failure.} The 2.33pp drop on POPE-random (86.30 to 83.97) is the price of the residual-stream perturbation that comes with keeping the prefix tokens in the sequence. Since the RMS-prefix configuration is the only one that gives strong OOD spatial signal (VSR 60.01\%, main paper Table~6), the trade is worth flagging but not framing as a failure of the design.

% =====================================================
\section{Extended Discussion}
\label{supp:sec:discussion}
% =====================================================

This section extends the Conclusion of the main paper with the four discussion threads that space did not permit in the main text.

\noindent\textbf{What would a non-suppressed injection look like?}
Suppression arises from two interacting causes: (i)~the auxiliary signal is caption-invariant, so the discriminative gradient through the gate is approximately zero, and (ii)~the task loss treats the signal as noise. A pathway that avoids both properties would need to be \emph{text-coupled}: its contribution to the hidden states should depend on the text being processed, not only on the image. Query-conditioned bilinear interactions between text queries and geometric features are a natural candidate. Since each preposition (``on,'' ``under,'' ``beside'') would then obtain a different lens onto the relational structure, the pathway would carry the first-order gradient that caption-invariant injections lack.

\noindent\textbf{Why geometry helps training but not inference.}
The geometric losses (IoA-driven entailment, angular repulsion) shape LoRA weight updates during training by providing a structured auxiliary objective that prevents overfitting to surface patterns of the training set. LoRA fine-tuning without auxiliary supervision has been reported to move GQA accuracy below the pretrained baseline~\cite{hypervis2026}; with the geometric losses in place, accuracy is preserved or improved across every configuration we tested. This regularisation effect does not require the geometric signal to be useful at inference. It acts through the training dynamics, not the inference pathway.

\noindent\textbf{The compositionality--generation tradeoff is partly a norm tradeoff.}
Unnormalised prefix tokens force the LLM to attend to them by virtue of their large magnitude, which benefits log-likelihood scoring but disrupts autoregressive generation. RMS normalization trades some of this forced-attention compositional signal for generation safety: the prefix tokens remain in the sequence but no longer dominate the attention distribution.

\noindent\textbf{Implications beyond this work.}
Suppression is not specific to hyperbolic geometry, nor even to visual relational signals. Any auxiliary pathway controlled by a learnable gate and trained under a task loss that does not directly reward the pathway's contribution will be subject to it. This covers adapters, side-networks, and external-memory injection mechanisms alike. The practical implication follows: beneficial signals should be injected non-optionally, with the engineering (scale matching, norm alignment) done correctly, rather than delegated to a learnable gate that the optimizer will close.

\noindent\textbf{Connection to the residual-stream literature.}
The residual-stream-dominance argument in the main paper's Sec.~4 rests on a standard reading from mechanistic interpretability: transformer hidden states can be read as a sum of contributions written by earlier blocks and never explicitly subtracted. The 36$\times$ initial-norm gap is a large-perturbation instance of the same phenomenon that mechanistic-\allowbreak interpretability studies observe at smaller scales when they inspect the ``residual stream'' at intermediate layers. In our setting the effect is loud enough that a simple RMS rescaling suffices to restore generation quality; more subtle norm mismatches, which are common across VLM adapter architectures, may be silent contributors to reported generation degradations.

% =====================================================
\section{Limitations}
\label{supp:sec:limitations}
% =====================================================

The main paper's Conclusion summarises the caveats in one sentence and points here. This section expands each into a paragraph and, at the end, tabulates the follow-up experiments that we did not run within the sprint budget for this submission.

\noindent\textbf{Single-seed training.} Every configuration in this paper is a single training run under one fixed seed. Test-time bootstrap CIs quantify evaluation noise but not training noise; the rel/attr dissociation reported in the main paper therefore rests on one run per configuration. Characterising training-seed variance for the headline configurations (soft-prompt, RMS-prefix, attention-bias, synthesis) is the most important reliability check we do not report.

\noindent\textbf{Scope of Proposition~1 of the main paper.} The proposition establishes that the \emph{first-order} discriminative gradient through the gate vanishes under caption-invariance. It does not by itself imply gate stalling: as S3 demonstrates, systematic second-order effects can drive the gate strongly. Our second-order account (Regime B in the main paper) is descriptive rather than formal. A formal second-order analysis of when auxiliary perturbations systematically hurt the loss remains open.

\noindent\textbf{Scope of the noise-regularisation control.} The G2 ablation in the main paper removes the geometric \emph{losses} but keeps the hyperbolic architecture and training recipe. This isolates the loss contribution from the architecture contribution, but does not rule out the stronger NEFTune-style hypothesis~\cite{jain2024neftune} that random-noise embeddings could substitute for the entire injection pathway. A fixed-random-prefix control, identical recipe, random-tensor prefix in place of the hyperbolic graph, would tighten this. We did not run it within the sprint budget for this submission.

\noindent\textbf{Task-format and backbone scope.} We evaluate on LLaVA-1.5-7B only, so the suppression phenomenon should be tested on other VLM families and scales. The trade-off avoidance claim is a within-fine-tuned-regime statement: on out-of-distribution VSR (main paper), all GQA-tuned configurations underperform vanilla, and only the geometric-\emph{prefix} configuration corroborates trade-off avoidance out-of-domain; the attention-bias configuration does not. Extending training to include diverse spatial data may close the vanilla-vs.-fine-tuned gap.

\noindent\textbf{Non-hyperbolic auxiliary signals.} The mechanism-level suppression claim generalises beyond hyperbolic geometry (Sec.~\ref{supp:sec:discussion}), but we do not test that generalisation directly. A non-geometric structured signal --- e.g., a scene-graph-derived attention bias --- injected through the same gated pathway would test whether suppression is truly signal-agnostic.

\begin{table}[t]
\centering
\caption{Follow-up experiments deferred to future work.}
\label{supp:tab:futurework}
\scalebox{0.88}{
\begin{tabular}{p{0.45\linewidth}p{0.48\linewidth}}
\toprule
\textbf{Experiment} & \textbf{What it would establish} \\
\midrule
Multi-seed training for the 4 headline configurations & Training-seed variance for the rel/attr dissociation \\
Fixed-random-prefix control (NEFTune-strength test) & Whether random-noise substitutes for the hyperbolic prefix \\
Text-coupled bilinear injection & Whether breaking caption-invariance breaks the dead-gradient regime \\
Paired-bootstrap test on shared 5{,}308 rel questions & Whether the CI-overlaps in the rel-preservation claim reach significance under a paired test \\
LLaVA-1.5-13B / Qwen-VL / Idefics backbones & Whether suppression is LLaVA-specific or general to instruction-tuned VLMs \\
Non-hyperbolic structured signals (scene graphs, dense predictions) & Whether the suppression finding is truly signal-agnostic \\
\bottomrule
\end{tabular}}
\end{table}

% \bibliographystyle{splncs04}
% \bibliography{main}

\end{document}
